# Supplementary material for: Lower Bounds for Adversarially Robust PAC Learning
Source: arXiv:1906.05815 source file (2019-06-13)
Supplement: Supplementary file 1 [file appendix.tex]

\section*{Supplemental Material}
\section{Preliminaries}

In Section \ref{sec:defs} we proposed definitions of PAC learning under evasion, poisoing, and hybrid attacks. They are all extensions of the following basic form of PAC learning \citep{Valiant:PAC}.
\begin{definition}[Realizable PAC Learning]\label{def:pac}
%\Dnote{Do we want to restrict the definition to realizable problems only?} \Mnote{I prefer not, because it is a nontrivial assumption that does not hold for many interesting cases.} 
A realizable classification problem $\problem_n=(\XX,\YY,\D,\C,\H)$ is PAC learnable with sample complexity $\SamCom(\eps,\delta,n)$ if there is a  learning algorithm $L$ such that for every $n$, $0<\eps,\delta<1$, $c \in \C$,  $D\in\D$, if we let $m=\SamCom(\eps,\delta,n)$, it holds that, 
$$\Pr_{\substack{\train \gets (D,c(D))^m, h \gets L(\train)}}[\Risk(D, c,h) \leq \eps] \geq 1-\delta.$$
We say $L$ has \emph{polynomial sample complexity} if $\SamCom(\eps,\delta,n) = \poly(n/\eps \delta)$, and is \emph{efficient} if it runs in time $\poly(n/\eps \delta)$.  
\end{definition}
The definition above leads to the ``standard'' form of \emph{distribution-independent} PAC learning by letting $\D$ to contain all distributions over $\XX$. We are particularly interested in distribution-specific cases as well, because our main results are \emph{negative} results on PAC learning; restricting $\D$ in those cases makes the results stronger.
%\Mnote{Also note on why we ignore realizability and agnostic cases? or pac learning of regression} 

%\section{Proofs of   Theorem \ref{thm:main} and Lemma \ref{lem:main}} \label{sec:proofs}
